# Supplementary material for: Resolving Dispersion and Induction Components for Polarisable Molecular Simulations of Ionic Liquids
Source: arXiv:1703.01540 source file (2017-05-02)
Supplement: Supplementary file 1 [file suppinfo.pdf]

# Resolving Dispersion and Induction Components for Polarisable Molecular Simulations of Ionic Liquids.
# Supplementary Information

Agílio A. H. Pádua*

*Institute of Chemistry of Clermont-Ferrand,*

*Universté Clermont Auvergne & CNRS, 63000 Clermont-Ferrand, France*

(Dated: May 2, 2017)

* agilio.padua@uca.fr

TABLE S1. Energetic quantities used in the calculation of the cohesive energy terms from molecular dynamics trajectories, including trajectory-averaged energy components for the ionic liquid and for the isolated ions. Total energy (including intramolecular terms), Lennard-Jones energy and electrostatic energy (including long-range part) are given. FixQ: integer fixed-charge CL&P force field; Drude: polarisation added to the CL&P model; SDrude: polarisation with scaled-down LJ $\epsilon_{ij}$.

| $\mathrm{kJ\,mol^{-1}}$ | $\frac{\langle E^{\mathrm{LI}}\rangle}{N}$ | $\frac{\langle E^{\mathrm{LI}}_{\mathrm{LJ}}\rangle}{N}$ | $\frac{\langle E^{\mathrm{LI}}_{\mathrm{elst}}\rangle}{N}$ | $\langle E^{+}\rangle$ | $\langle E^{+}_{\mathrm{LJ}}\rangle$ | $\langle E^{+}_{\mathrm{elst}}\rangle$ | $\langle E^{-}\rangle$ | $\langle E^{-}_{\mathrm{LJ}}\rangle$ | $\langle E^{-}_{\mathrm{elst}}\rangle$ |
|---|---|---|---|---|---|---|---|---|---|
| $[C_2C_1im][dca]$ 303 K | | | | | | | | | |
| FixQ | −244.9 | −73.6 | −304.8 | 245.7 | −0.9 | 141.8 | 10.8 | −0.5 | −16.8 |
| Drude | −253.1 | −69.3 | −341.2 | 193.6 | −1.7 | 126.8 | 3.1 | −0.5 | −23.2 |
| SDrude | −238.5 | −48.0 | −351.3 | 193.6 | −1.7 | 126.8 | 3.1 | −0.5 | −23.2 |
| $[C_4C_1im][Ntf_2]$ 323 K | | | | | | | | | |
| FixQ | 112.1 | −124.3 | −31.8 | 299.9 | −1.2 | 150.4 | 305.8 | −5.7 | 192.6 |
| Drude | 94.7 | −119.9 | −91.5 | 229.9 | −2.3 | 120.1 | 287.8 | −5.3 | 153.2 |
| SDrude | 124.4 | −89.2 | −93.8 | 221.3 | −2.1 | 119.9 | 287.8 | −5.3 | 153.2 |
| $[C_4C_1pyr][Ntf_2]$ 343 K | | | | | | | | | |
| FixQ | 306.3 | −96.1 | 15.1 | 487.8 | 24.1 | 195.0 | 312.5 | −5.5 | 192.5 |
| Drude | 286.9 | −92.7 | −46.3 | 399.3 | 18.0 | 152.2 | 295.0 | −4.9 | 153.4 |
| SDrude | 329.8 | −48.4 | −48.8 | 389.8 | 17.1 | 153.0 | 295.0 | −4.9 | 153.4 |

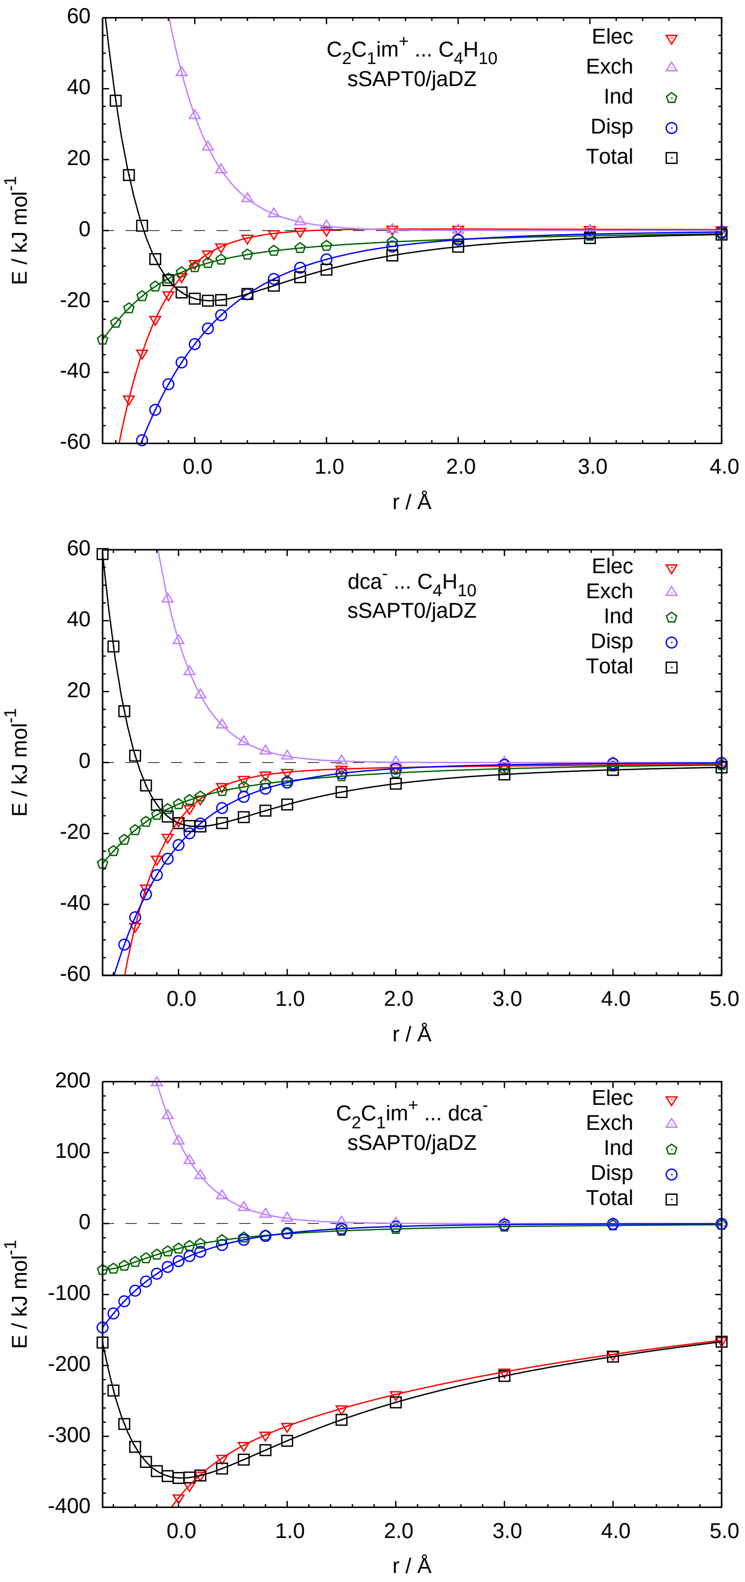


FIG. S1. Decomposition of the potential energies of interaction involving dimers of $C_2C_1im^+$, dca$^-$ and $C_4H_{10}$ from sSAPT0/jaDZ. The distances are measured from the potential energy minima and the orientations were kept fixed from the optimized dimer. The lines are just guides to the eye.

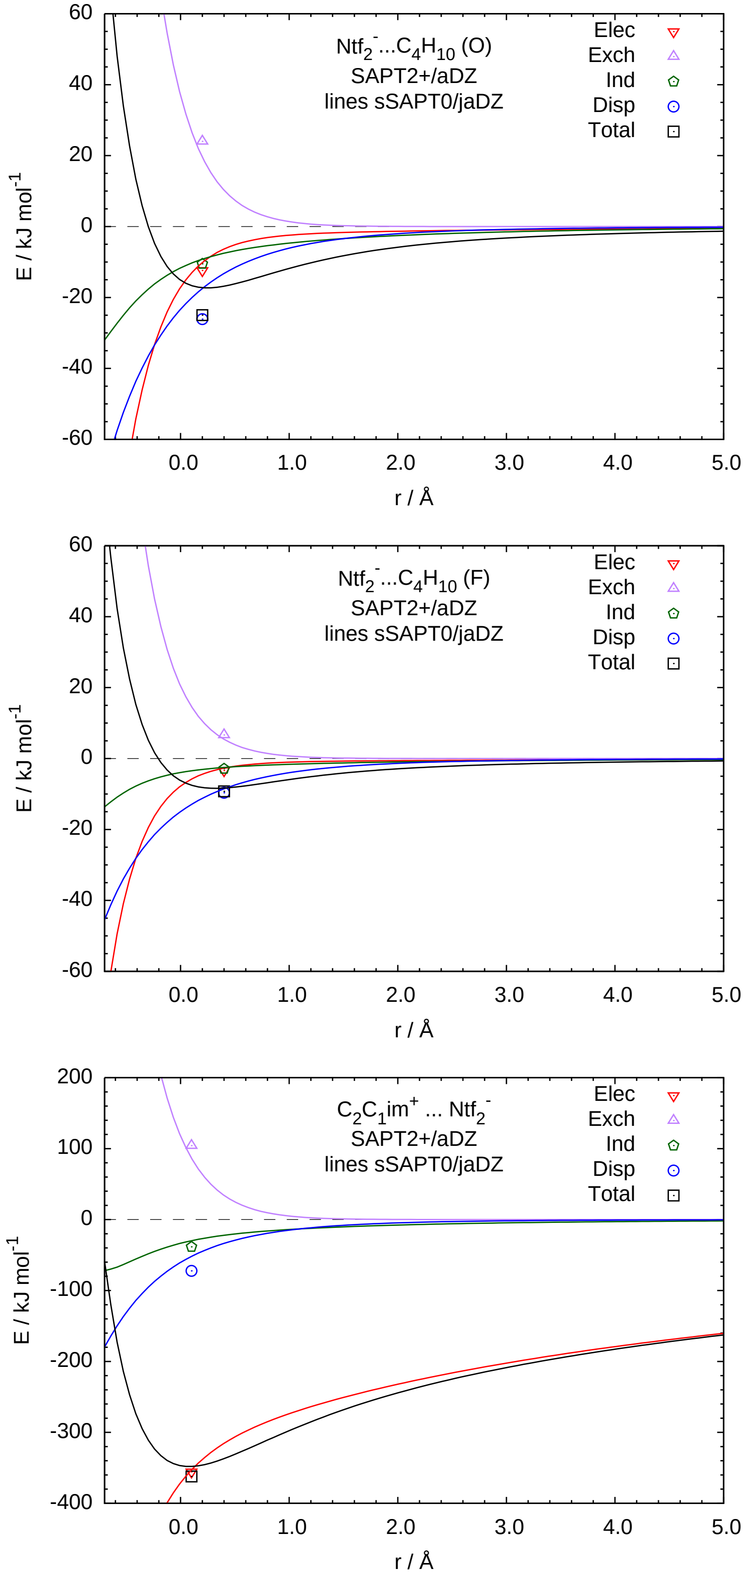


FIG. S2. Decomposition of the potential energies of interaction involving dimers of $C_2C_1im^+$, $Ntf_2^-$ and $C_4H_{10}$ from SAPT0/jaDZ and SAPT2+/aDZ, the latter at the equilibrium geometry. In the top plot the anion has the O atoms closer to the hydrocarbon, whereas in the middle plot the F atoms are closer.

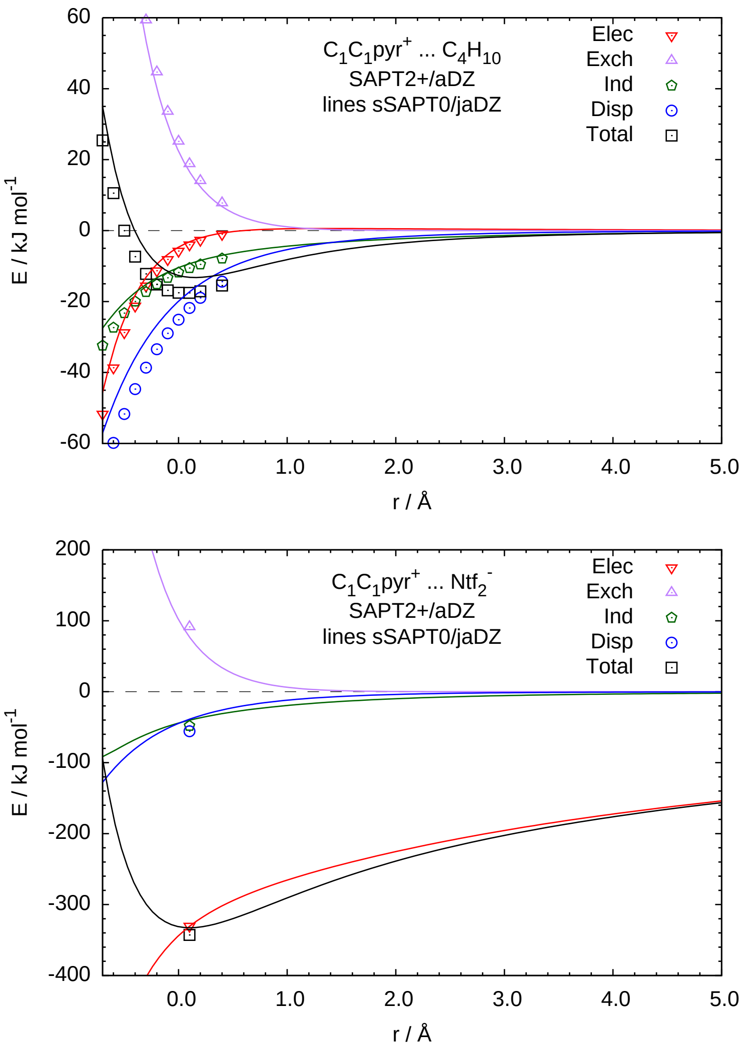


FIG. S3. Decomposition of the potential energies of interaction involving dimers of $C_1C_1pyr^+$, $Ntf_2^-$ and $C_4H_{10}$ from sSAPT0/jaDZ and SAPT2+/aDZ.

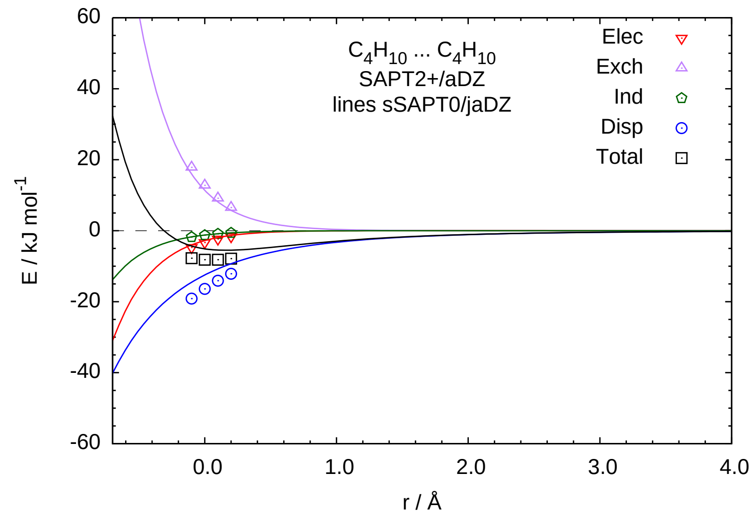


FIG. S4. Decomposition of the potential energies of interaction between $C_4H_{10}$ dimers from sSAPT0/jaDZ and SAPT2+/aDZ.

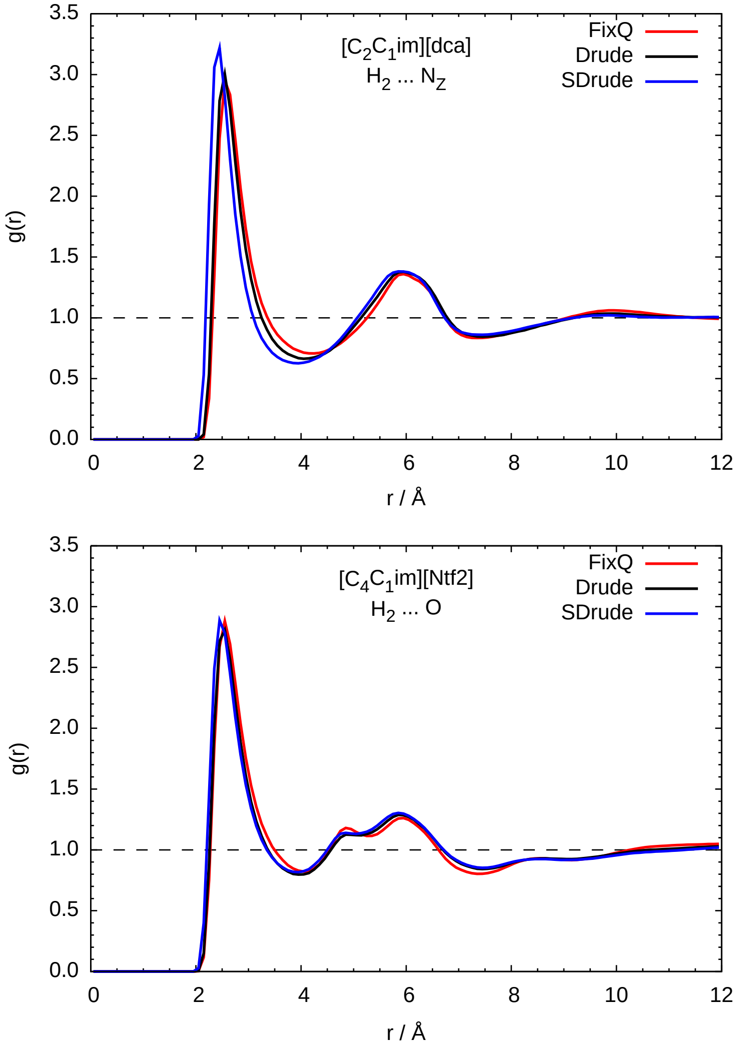


FIG. S5. Radial distribution functions between $H_2$ atoms of the cation and the $N_Z$ atoms of the anion in $[C_2C_1im][dca]$ at 303 K, or the O atoms of the anion in $[C_4C_1im][Ntf_2]$ at 323 K.
